# Supplementary material for: Weak anti-localization of two-dimensional holes in germanium beyond the diffusive regime
Source: arXiv:1807.01400 ancillary file (2018-07-03)
Supplement: Supplementary file 1 [file Supplementary_Information.pdf]

# Supplementary Information

## I. NUMERICAL EVALUATION OF THE CONDUCTANCE CORRECTION DUE TO WEAK LOCALIZATION

Our goal is to evaluate integrals of three related forms from [M. M. Glazov and L. E. Golub, Semiconductors **40**, 1209 (2006)][1] that were originally written as

$$\begin{aligned} P_N &= \frac{l_B}{l}\int_0^\infty dx \exp\left(-\frac{l_B}{\tilde{l}}x - \frac{x^2}{2}\right) L_N^0(x^2), \\ Q_N &= \frac{1}{\sqrt{N+1}}\frac{l_B}{l}\int_0^\infty dx \exp\left(-\frac{l_B}{l}x - \frac{x^2}{2}\right) x L_N^1(x^2), \\ R_N^{(m)} &= \frac{l_B}{l\sqrt{2}}\sqrt{\frac{N!}{(N+m)!}}\int_0^\infty dx \exp\left(-\frac{l_B}{l}x - \frac{x^2}{2}\right) x^m L_N^m(x^2)\sin\left(2\Omega\tau\frac{l_B}{l}x\right), \\ S_N^{(m)} &= \frac{l_B}{l}\sqrt{\frac{N!}{(N+m)!}}\int_0^\infty dx \exp\left(-\frac{l_B}{l}x - \frac{x^2}{2}\right) x^m L_N^m(x^2)\sin^2\left(\Omega\tau\frac{l_B}{l}x\right), \end{aligned}$$

where $L_N^m(x)$ are generalized Laguerre polynomials. For large $N$ values, it is difficult to evaluate these polynomials numerically, and cancellations between small and large values in the polynomial and exponential terms at large $x$ can cause additional numerical problems. Before continuing with integral evaluations, we redefine these integrals in terms of a simple parent integral,

$$\begin{aligned} F_n^m(q) &\equiv \sqrt{\frac{n!}{(n+m)!}}\int_0^\infty dx \exp\left(-qx - \frac{x^2}{2}\right) x^m L_n^m(x^2), \quad (1) \\ P_N &= \frac{l_B}{l}F_N^0\left(\frac{l_B}{l}\frac{l}{\tilde{l}}\right), \\ Q_N &= \frac{l_B}{l}F_N^1\left(\frac{l_B}{l}\right), \\ R_N^{(m)} &= \frac{l_B}{l\sqrt{2}}\mathrm{Im}\left[F_N^m\left(\frac{l_B}{l}(1-2\Omega\tau i)\right)\right], \\ S_N^{(m)} &= \frac{l_B}{2l}\mathrm{Re}\left[F_N^m\left(\frac{l_B}{l}\right) - F_N^m\left(\frac{l_B}{l}(1-2\Omega\tau i)\right)\right]. \end{aligned}$$

We can rewrite $F_n^m(q)$ in a more convenient way by using some of the orthogonal-polynomial structure of the generalized Laguerre polynomials. The weight function that defines their orthogonality is

$$w_m(x) = x^m e^{-x} \quad \text{for} \quad x \in [0,\infty), \quad (2)$$

and it is common to combine orthogonal polynomials with their weight functions and normalization factors to define a convenient orthonormal basis,

$$g_n^m(x) \equiv \sqrt{\frac{n!}{(n+m)!}}\sqrt{w_m(x)}L_n^m(x). \quad (3)$$

In terms of these functions, the integral reduces to an integral between a Laguerre basis function and a complex exponential,

$$F_n^m(q) = \int_0^\infty dx \exp(-qx) g_n^m(x^2). \quad (4)$$

The inner product between Laguerre basis functions is

$$\langle f, g\rangle = \int_0^\infty dx f(x) g(x). \quad (5)$$

We will evaluate these two types of integrals numerically with a common quadrature, to be determined.

The other important numerical ingredient is the stable evaluation of $g_n^m$. The polynomials are defined by a three-term recursion relation,

$$L_0^m(x) = 1, \tag{6}$$
$$L_1^m(x) = 1 + m - x, \tag{7}$$
$$L_{n+1}^m(x) = \frac{(2n+1+m-x)L_n^m(x) - (n+m)L_{n-1}^m(x)}{n+1}. \tag{8}$$

This can be adapted into a three-term recursion relation for $g_n^m$,

$$g_0^m(x) = \sqrt{\frac{w_m(x)}{m!}}, \tag{9}$$
$$g_1^m(x) = \frac{g_0^m(x)}{\sqrt{m+1}}(1+m-x), \tag{10}$$
$$g_{n+1}^m(x) = \frac{(2n+1+m-x)\sqrt{\frac{n+1}{n+m+1}}g_n^m(x) - (n+m)\sqrt{\frac{(n+1)n}{(n+m+1)(n+m)}}g_{n-1}^m(x)}{n+1}. \tag{11}$$

These recurrence relations are not necessarily numerically stable, and require numerical evaluations of the inner product to check orthogonality and perform Gram-Schmidt orthogonalization.

The final ingredient of a numerical method is a quadrature rule. To make this process as straightforward as possible, we map the $[0,\infty)$ domain to $(-\infty,\infty)$ and use a uniform quadrature defined by a grid spacing and upper and lower cutoff values. We use the variable $y = \ln(e^x - 1)$ in Eq. (4) and $z = \ln(e^{\sqrt{x}} - 1)$ in Eq. (5),

$$F_n^m(q) = \int_{-\infty}^{\infty} \frac{dy}{1+e^{-y}} \exp[-q\ln(e^y+1)] g_n^m[\ln^2(e^y+1)], \tag{12}$$
$$\langle f, g\rangle = \int_{-\infty}^{\infty} \frac{2\ln(e^z+1)dz}{1+e^{-z}} f[\ln^2(e^z+1)] g[\ln^2(e^z+1)]. \tag{13}$$

With the inner product available, we can test the numerical stability of the three-term recurrence as measured by a loss of orthogonality. From initial numerical tests, the recurrence in terms of $g_n^m$ appears to be stable and loss of orthogonality seems to be related to some combination of quadrature errors and underflow to zero in the simple recurrence implementation.

The intended application of these integrals contains an infinite sum over $n$ for $F_n^m(q)$ and this sum is very slow to converge in some parameter regimes, particularly when $\mathrm{Re}(q)$ is large and the $1/q$ suppression of the integrals is offset by a $q$ prefactor. In this limit, the exponential behaves like a delta function, and only $P_n$ has a nonzero asymptotic value that we derive from the asymptotic expansion of the Laguerre polynomials as Bessel functions of the first kind, $J_0(x)$, for large $n$ as

$$P_n \approx \frac{l_B}{l} \int_0^{\infty} dx J_0(2\sqrt{n}x) = \frac{l_B}{2l\sqrt{n}}. \tag{14}$$

The first-order asymptotic correction to $\sigma_a$ in Eq. (35) of the original paper is

$$\sigma_a = -\frac{e^2}{2\pi^2\hbar}\left(\frac{l}{l_B}\right)^2 \left[\sum_{n=0}^{n_{\max}-1}(\cdots) + 2\sum_{n=n_{\max}}^{\infty} P_n^3\right] \tag{15}$$
$$= -\frac{e^2}{2\pi^2\hbar}\left(\frac{l}{l_B}\right)^2 \left[\sum_{n=0}^{n_{\max}-1}(\cdots) + \frac{1}{4}\left(\frac{l_B}{l}\right)^3 \sum_{n=n_{\max}}^{\infty}\frac{1}{n^{1.5}}\right] \tag{16}$$

and the accompanying $\sigma_b$ in Eq. (37) does not have any terms that converge as slowly. The infinite sum can be grouped into a finite sum and an evaluation of the Riemann zeta function, $\zeta(x)$, as

$$\sum_{n=n_{\max}}^{\infty}\frac{1}{n^{1.5}} = \zeta(1.5) - \sum_{n=1}^{n_{\max}-1}\frac{1}{n^{1.5}} \approx 2.6124 - \sum_{n=1}^{n_{\max}-1}\frac{1}{n^{1.5}}. \tag{17}$$

Adding this correction helps to converge calculations for large $l_B/l$. It is possible to construct a more general asymptotic expansion that expands all the integrals in powers of $1/\sqrt{n}$ and reduce all integral to moments of Bessel functions. This is necessary to thoroughly converge the infinite summations over $n$.

To evaluate the asymptotic expansions, we first define the function

$$j_m(\alpha,\beta) = \int_0^\infty \mathrm{d}u\ J_m(\alpha u) e^{-(1-i\beta)u} \tag{18}$$

$$= \frac{\alpha^m}{(1-i\beta)^{m+1}} \frac{\left(1+\sqrt{1-\frac{\alpha^2}{(i+\beta)^2}}\right)^{-m}}{\sqrt{1-\frac{\alpha^2}{(i+\beta)^2}}}, \tag{19}$$

where $J_m$ is the Bessel function of the first kind. We obtain the following asymptotic expansions in terms of $j_m$:

$$P_N \approx \frac{\tilde{l}}{l} j_0(2\sqrt{N}\frac{\tilde{l}}{l_B}, 0) \tag{20}$$

$$Q_N \approx \sqrt{\frac{N}{N+1}} j_1(2\sqrt{N}\frac{l}{l_B}, 0) \tag{21}$$

$$R_N^{(m)} \approx \frac{1}{\sqrt{2}} \sqrt{\frac{N!}{(N+m)!}} N^{m/2}\ \mathrm{Im}\big[j_m(2\sqrt{N}\frac{l}{l_B}, 2\Omega\tau)\big] \tag{22}$$

$$S_N^{(m)} \approx \frac{1}{2} \sqrt{\frac{N!}{(N+m)!}} N^{m/2}\Big[j_m(2\sqrt{N}\frac{l}{l_B}, 0) - \mathrm{Re}\big[j_m(2\sqrt{N}\frac{l}{l_B}, 2\Omega\tau)\big]\Big] \tag{23}$$

In our evaluation of the conductance shift, we have switched from computing the integrals directly with $10^4$ quadrature points to evaluating the asymptotic expressions for $N \geq 100$ and have truncated the sums for $\sigma_a$ and $\sigma_b$ at $N = 10^4$.

To perform fits to the experiment, we first performed an evaluation of the conductance shift $\Delta\sigma = \sigma_a + \sigma_b$ over a 2d grid of values of $\tau_\phi$ and $\tau_{\mathrm{SO}}$ over a range of B-field values in the interval [0.1, 10] mT. We then compared these $\Delta\sigma(B)$ curves to postprocessed experimental data to obtain a misfit for each of the $(\tau_\phi, \tau_{\mathrm{SO}})$ parameter values. We provide all code used to perform the postprocessing and numerical evaluation of the conductance shift in the included supplementary software files.

## II. FITTING WITH THE HLN MODEL

We use the HLN model[2] to fit the magneto-resistance curves:

$$\begin{aligned} &\Delta\sigma(B) - \Delta\sigma(0) \\ &= \frac{e^2}{2\pi^2\hbar}\Big\{\Psi\Big(\frac{1}{2}+\frac{B_\phi}{B}+\frac{B_{SO}}{B}\Big) + \frac{1}{2}\Psi\Big(\frac{1}{2}+\frac{B_\phi}{B}+\frac{2B_{SO}}{B}\Big) - \frac{1}{2}\Psi\Big(\frac{1}{2}+\frac{B_\phi}{B}\Big) \\ &- ln\frac{B_\phi+B_{SO}}{B} - \frac{1}{2}ln\frac{B_\phi+2B_{SO}}{B} + \frac{1}{2}ln\frac{B_\phi}{B}\Big\} \end{aligned} \tag{24}$$

The fitting range is -10 mT to 10 mT. The data points within -3 mT to 3 mT are weighted by a factor of 20 to keep the region that contains the most information (theWL to WAL crossover point) fit well. The fitting gives the spin relaxation time $\tau_{relax} = \hbar/(4eDB_{SO})$, which is different from the spin precession time $\tau_{SO}$. The energy splitting $\Delta_{SO}$ is obtained by relating $\tau_{relax}$ with $\Omega_3$ through the D'yakonov-Perel' spin relaxation mechanism: $1/\tau_{relax} = 2|\Omega_3|^2\tau_3$. It is assumed that the scattering is isotropic, which gives $\tau_3 = \tau_1 = \tau_{tr}$, where $\tau_n = \int d\theta W(\theta)(1-cos(n\theta))$, and $W(\theta)$ is the scattering probability density.


[1] M. M. Glazov and L. E. Golub, Semiconductors **40**, 1209 (2006).

[2] S. Hikami, A. I. Larkin, and Y. Nagaoka, Progr. Theor. Exp. Phys. **63**, 707 (1980).
